# Supplementary material for: Instructing the Architecture Search for Spatial-temporal Sequence Forecasting with LLM
Source: arXiv:2503.17994 source file (2025-03-23)
Supplement: Supplementary file 1 [file method_details.tex]

\section{Details of Search Space}
\label{app-vis-stcell}
\subsection{Spatial Operator}
Following \cite{AutoST}, we define the spatial operator as follows:
\begin{equation}
    \text{MG}(X, A, ord) 
    = \begin{cases}
	X, & ord = 0\\
	\text{MixGC}(X, A), & ord = 1 \\
        \text{MixGC}(H^{(ord - 1)}A) & ord > 1
		   \end{cases},
\end{equation}
where 
\begin{equation}
\begin{aligned}
\text{MixGC}(X, A) = \text{ChebNet}(X, A) + \text{AdapDC}(X, A) \\
 = \hat{A}XW_g + P_fXW_f + P_bXW_b + \hat{A}_{adp}XW_{adp},
\end{aligned}
\end{equation}
which are proposed in ChebNet\cite{ChebNet} and GraphWaveNet\cite{GraphWaveNet}. The spatial connections of nodes are descriped by $\hat{A} = D^{1/2}\Tilde{A}D^{1/2}$, where $\Tilde{A} = A + 1$, and $D_{ii} = \sum_j \Tilde{A}_{ij}$. And $P_f = A / \text{rowsum}(A)$, $P_b = A^\text{T} / \text{rowsum}(A^\text{T})$, $\hat{A}_{adp} = \text{Softmax}(\text{RELU}(E_1 E_2^\text{T}))$. The  $E_1, E_2 \in \mathbb{R}^{N \times C}$ are learnable node embedding matrices.  

\subsection{Temporal Operator}

Following POLLA\cite{Pola}, we use the technique of linear self-attention as the temporal operator.
\begin{equation}
    \text{LA}(Q, K, V) = \phi(Q) \big(\phi(K) ^\text{T} V\big),
\end{equation}
where $Q = XW_Q, K = XW_K, V = XW_V$, $W_Q$, $W_K$, $W_V$ are learnable matrices. Compared with traditional self-attention mechanism, linear self-attention is more efficient in computing. 
\subsection{ST-cells}

In our method, ST-cell is the basic search unit of the search process. Following AutoST\cite{AutoST}, we include three types of ST-cells, namely spatial-first cell, temporal-first cell and spatial-temporal-synchronous cell. The formulated definition is given below. 

The spatial-first cell is formulated as follows:

\begin{equation}
\begin{aligned}
     Y_{\mathrm{S-First}} = \mathrm{FFN}\Big(\mathrm{T}\big(\mathrm{S}(X)\big)\Big) \\
     = \mathrm{FFN}\Big(\text{LA}(Q, MG_1, MG_2)\Big),
\end{aligned}
\end{equation}
where $Q = XW_Q$, $MG_1 = \text{MG}(X, A, ord)W_K$, and $MG_2 = \text{MG}(X, A, ord)W_V$. 

The Temporal-first cell is formulated as follows:
\begin{equation}
\begin{aligned}
    Y_{\mathrm{T-First}} = \mathrm{FFN}\Big(\mathrm{S}\big(\mathrm{T}(X)\big)\Big) \\
     = \mathrm{FFN}\Big(\text{MG}(\text{LA}(Q, K, V), A, ord)\Big),
\end{aligned}
\end{equation}
where $Q = XW_Q$, $K = XW_K$, and $V = XW_V$. 

The spatial-temporal-synchronous cell is formulated as follows:
\begin{equation}
\begin{aligned}
    Y_{\mathrm{ST-Syn}} = \mathrm{FFN}\Big(\mathrm{concat}\big(\mathrm{S}(X), \mathrm{T}(X)\big)\Big)\\
    = \mathrm{FFN}\Big(\mathrm{concat}[\text{LA}(Q, K, V), \text{MG}(X, A, order)]\Big),
\end{aligned}
\end{equation}
where $Q = XW_Q$, $K = XW_K$, and $V = XW_V$. The $\mathrm{concat}$ method is to combine the two type operators. 

\begin{figure}
	\centering

		\centering
		\includegraphics[width=\linewidth]{figs/method/cells-2.png}
		\caption{The three kinds of ST-cells, including spatial-first cells, temporal-first cells, and spatial-temporal synchronous cells, capture various ST dependencies. 
        }
		\label{ST-Cells}%文中引用该图片代号

\end{figure}

\subsection{Assembly Architecture}
Figure \ref{Cell} shows a search structure of neural architecture, with 4 nodes and 6 edges combining as a directed acyclic graph (DAG), where nodes denote hidden states and edges denote ST-cells. The ST-cell is defined as above, including spatial-first, temporal-first and spatial-temporal synchronous cells. We adopt the hybrid assembly search, following AutoST \cite{AutoST}, which provides a flexible way of complex architecture designing as the jumping and merging action can formulate more information.
\begin{figure}
	\centering
	
		\centering
		   \includegraphics[totalheight=1.6in]{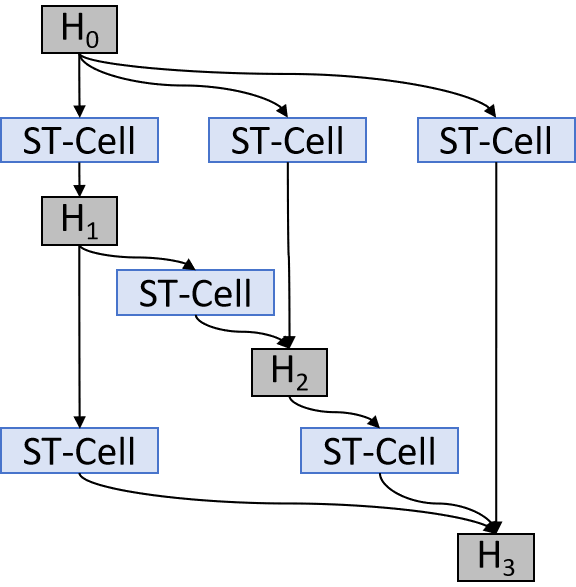}
              \caption{Hybrid Assembly Structure.
                The structure is built into a DAG, with 6 operation cells. %and each cell can be one of three kinds of ST-cells.
              }
            \label{Cell}

\end{figure}
